# Supplementary material for: VSAC: Efficient and Accurate Estimator for H and F
Source: arXiv:2106.10240 source file (2021-09-13)
Supplement: Supplementary file 1 [file supplementary.tex]

\clearpage
\section*{Supplementary material}
\subsection*{Linear P6P}
The advantages of GE applies as well when estimating the perspective projection $\textbf{P} \in \mathbb{R}^{3\times4}$ matrix. 
In the uncalibrated case, $\textbf{P}$ can be estimated from six 2D-3D correspondences using linear equations. The projection matrix is given up-to-scale and, hence, has 11 unknown parameters. 
Therefore, the estimation requires, in theory, 11 constraints from 5 and ``half'' correspondences since each one yields two equations. 
Since this means, in practice, that six correspondences need to be sampled,
the usual solution is the least-squares minimization via SVD, considering all the 12 equations or to apply the Jackknife method
As mentioned earlier, the speed of the estimation from a minimal sample is more important than its accuracy, due to being applied sometimes thousands of times.
Therefore, we propose to apply GE instead of SVD. Moreover, the matrix of linear equations for estimation of perspective projection contains a lot of zeros, hence similar techniques can be used as was done for homography in \cite{RHO}.
\subsection*{Parallel processing}
\subsection*{Ranking and points correction}
\subsection*{Final Optimization}
\noindent
\textbf{Final Optimization.} 
The proposed efficient iterative parameter polishing was compared to the single least squares approach on thousands of models, either estimated from the minimal sample or by the LO step. Two versions of the iterative LSQ were evaluated, (1) with normalization per iteration, (2) and with a single pre-normalization step plus covariance matrix update.
The data for homography fitting were taken from the \textsc{HPatches} dataset\footnote{\url{http://cmp.felk.cvut.cz/~mishkdmy/CVPR-RANSAC-Tutorial-2020/homography.tar.gz}} and, for fundamental matrix estimation, from \textsc{Kusvod2}\footnote{\url{http://lebeda.sk/DP/data/kusvod2.tar.gz}}. 

Table~\ref{table:lsq_res} reports the intermediate (\ie, in the current iteration of the LSQ fitting, shown by columns) average errors for 
the iterate-and-normalize method ($\varepsilon$), the errors of normalize-once ($\varepsilon'$) and the run-time ratio ($t/t'$), \ie, the speed-up caused by the proposed technique.
Errors for fundamental matrix is the same as in DEGENSAC experiments; for homography it is the average distance of projected points from the first frame to second by GT homography and the estimated one.
Results for homography are shown in the top block,
for fundamental matrix fitting in the bottom one.
\begin{table}[H]

\setlength{\tabcolsep}{5pt}
\begin{tabular}{|l|l|r|r|r|r|r|r|}
\hline
      \multicolumn{2}{|c|}{} & \multicolumn{1}{c|}{0} & \multicolumn{1}{c|}{1} & \multicolumn{1}{c|}{2} & \multicolumn{1}{c|}{3} & \multicolumn{1}{c|}{4}& \multicolumn{1}{c|}{5} \\ \hline\hline
\multirow{3}{*}{\rotatebox{90}{$H$}}&$\varepsilon$ & 1.120 & 0.718 & 0.648 & 0.627 & 0.618 & 0.612  \\ \cline{2-8}
&$\varepsilon^{\prime}$ & 1.120 & 0.718 & 0.648 & 0.627 & 0.617 & 0.612   \\ \cline{2-8}
&$t / t^{\prime}$ & - & 0.751 & 1.338 & 1.851 & 2.298 & 2.689  \\ \hline\hline
\multirow{3}{*}{\rotatebox{90}{$F$}}&$\varepsilon$ & 2.484 & 2.004 & 1.921 & 1.898 & 1.889 & 1.885 \\ \cline{2-8}
&$\varepsilon^{\prime}$ & 2.484 & 1.997 & 1.909 & 1.886 & 1.878 & 1.875 \\ \cline{2-8}
&$t / t^{\prime}$ & - & 0.894 & 1.140 & 1.263 & 1.335 & 1.384 \\ \hline
\end{tabular}
\vspace{-0.7em}
\caption{Final optimization on homographies ($H$) and fundamental matrices ($F$). 
Columns (0--5) show the results in the subsequent iterations of iterated LSQ. 
The average error (px) of the standard approach ($\varepsilon$) and the proposed one ($\varepsilon'$), run-time ratio ($t / t^{\prime}$ -- speed-up) of the standard fitting to the proposal are reported. Total number of tested final models  and average number of inliers for homography is 13,999 and 843; for fundamental matrix are 938 and 361, respectively.}
\label{table:lsq_res}
\end{table}
\subsection*{Parallel Processing}

Since each iteration in the original RANSAC runs almost independently on the previous ones, RANSAC can straightforwardly be parallelized.
However, this is not necessarily true for the state-of-the-art RANSAC alternatives since some algorithmic parts share common variables or proceed sequentially. 
To avoid the explicit communication among threads, it is better not to parallelize the main RANSAC loop but running several RANSACs in parallel. 
The modern libraries for parallelization enables to get a number of threads on a computer -- it is the upper bound of the number of RANSAC going to run in parallel. Each thread receives its own copy of the objects (\eg, sampler or minimal solver) and different states for the random generator. 
All threads run theirs own initialization of RANSAC sharing though only three atomic variables (safe in multithreading): counter of the number iterations done in total; a boolean variable that indicates termination for all threads if one of them found the solution; and the so-far-the-best number of inliers. 
Additionally, if PROSAC is used for sampling, there is one global sampler which is guarded by a mutex to ensure sequential sampling. 

%\todo{RANSAC in theory is never deterministic}
%Unfortunately, in these settings parallel RANSAC is non-deterministic -- because local optimization or SPRT has its own random generator, therefore the final result depends on how many times a thread was running. However, if PROSAC with no other extensions that require random generator is used then parallel version is deterministic. 

Parallel RANSAC is better to run on the hard problem, \ie, with a low inlier ratio. The observed speed-up is proportional to the number of cores. However, for high inlier ratio instances or PROSAC, the overhead for the creation of threads may exceed the time of the sequential version.

\subsection*{DEGENSAC}
\noindent
\textbf{DEGENSAC with calibration} was evaluated on image pairs from the CVPR IMW 2020 PhotoTourism challenge dataset\footnote{\url{https://vision.uvic.ca/image-matching-challenge/data/}} of Saint Peter's Square, which includes many images with the dominant plane of St.\ Peter's Basilica. 
For the experiments, we used three RANSAC variants, all of them combined with adaptive SPRT and LO. The only difference is that the first one uses the original DEGENSAC with a maximum of 20 iterations of the plane-and-parallax algorithm, the second uses 100 iterations, and the third applies the proposed calibrated DEGENSAC. 
The error is calculated as the average symmetric epipolar distance of the estimated epipolar geometry and the ground truth correspondences from the dataset. 
The same random seed was used for all algorithms, therefore, the results, inside the robust estimation procedure, start differing only after the first time when a degenerate model occurred.

Table~\ref{table:degen_res} reports the results on 1068 image pairs where DEGENSAC was used, \ie, were at least one degenerate minimum sample was detected.
Recovery of degenerate fundamental matrix of Calibrated DEGENSAC (DEG') is around 5 times faster than DEGENSAC with 20 iterations and 10 times faster than DEGENSAC with 100 iterations. 
% The average total time of RANSAC using new DEGENSAC is also lower. 
The right block of Table~\ref{table:degen_res} shows that the accuracy of the methods is similar.
\begin{table}[H]

\begin{tabular}{|l||r|r|r||r|r|r|}
\hline
       & \multicolumn{1}{c|}{$t^{R}_{\text{avg}}$} & \multicolumn{1}{c|}{$t^{D}_{\text{avg}}$} & \multicolumn{1}{c||}{$w^{t}_{\%}$} & \multicolumn{1}{c|}{$\varepsilon_{\text{avg}}$} & \multicolumn{1}{c|}{$\varepsilon_{\text{med}}$} & \multicolumn{1}{c|}{$w^{\varepsilon}_{\%}$} \\ \hline \hline
DEG$_{20}$ & 5.00 & 0.63 & 29.3 & {\bf 0.404} & 0.321 & 17.9 \\ \hline
DEG$_{100}$& 5.87 & 1.45 & 11.7 & 0.421 & 0.320 & 19.0 \\ \hline
DEG$^{\prime}$& {\bf 4.64} & {\bf 0.14} & {\bf 59.0} & 0.410 & {\bf 0.305} & {\bf 42.6} \\ \hline
\end{tabular}
\vspace{-0.7em}
\caption{
Comparison of the original DEGENSAC, using 20 and 100 max.\ iterations in the plane-and-parallax method, and the proposed one (DEG'). The average run-time in milliseconds of the entire robust estimation ($t^{R}_{\text{avg}}$); average time of recovering $F$ by DEGENSAC ($t^{D}_{\text{avg}}$); percentage of the cases when DEG' is the fastest; mean ($\varepsilon_{\text{avg}}$) and median ($\varepsilon_{\text{med}}$) errors; percentage of the cases when DEG' is the most accurate ($w^{\varepsilon}_{\%}$) are reported.}
\label{table:degen_res}
\end{table}
